# Supplementary material for: PolyFormer: Scalable Node-wise Filters via Polynomial Graph Transformer
Source: arXiv:2407.14459 source file (2024-07-19)
Supplement: Supplementary file 1 [file d_appendix.tex]

\section{Filters of PolyAttn} \label{filters_of_polyattn}
In this section, we present more illustrations of filters learned by PolyAttn on real-world datasets, as implemented in Section \ref{PolyAttn_on_realdata}.

\begin{figure}[htbp]
\centering
\begin{subfigure}{0.22\textwidth}
  \centering
  \includegraphics[width=\linewidth]{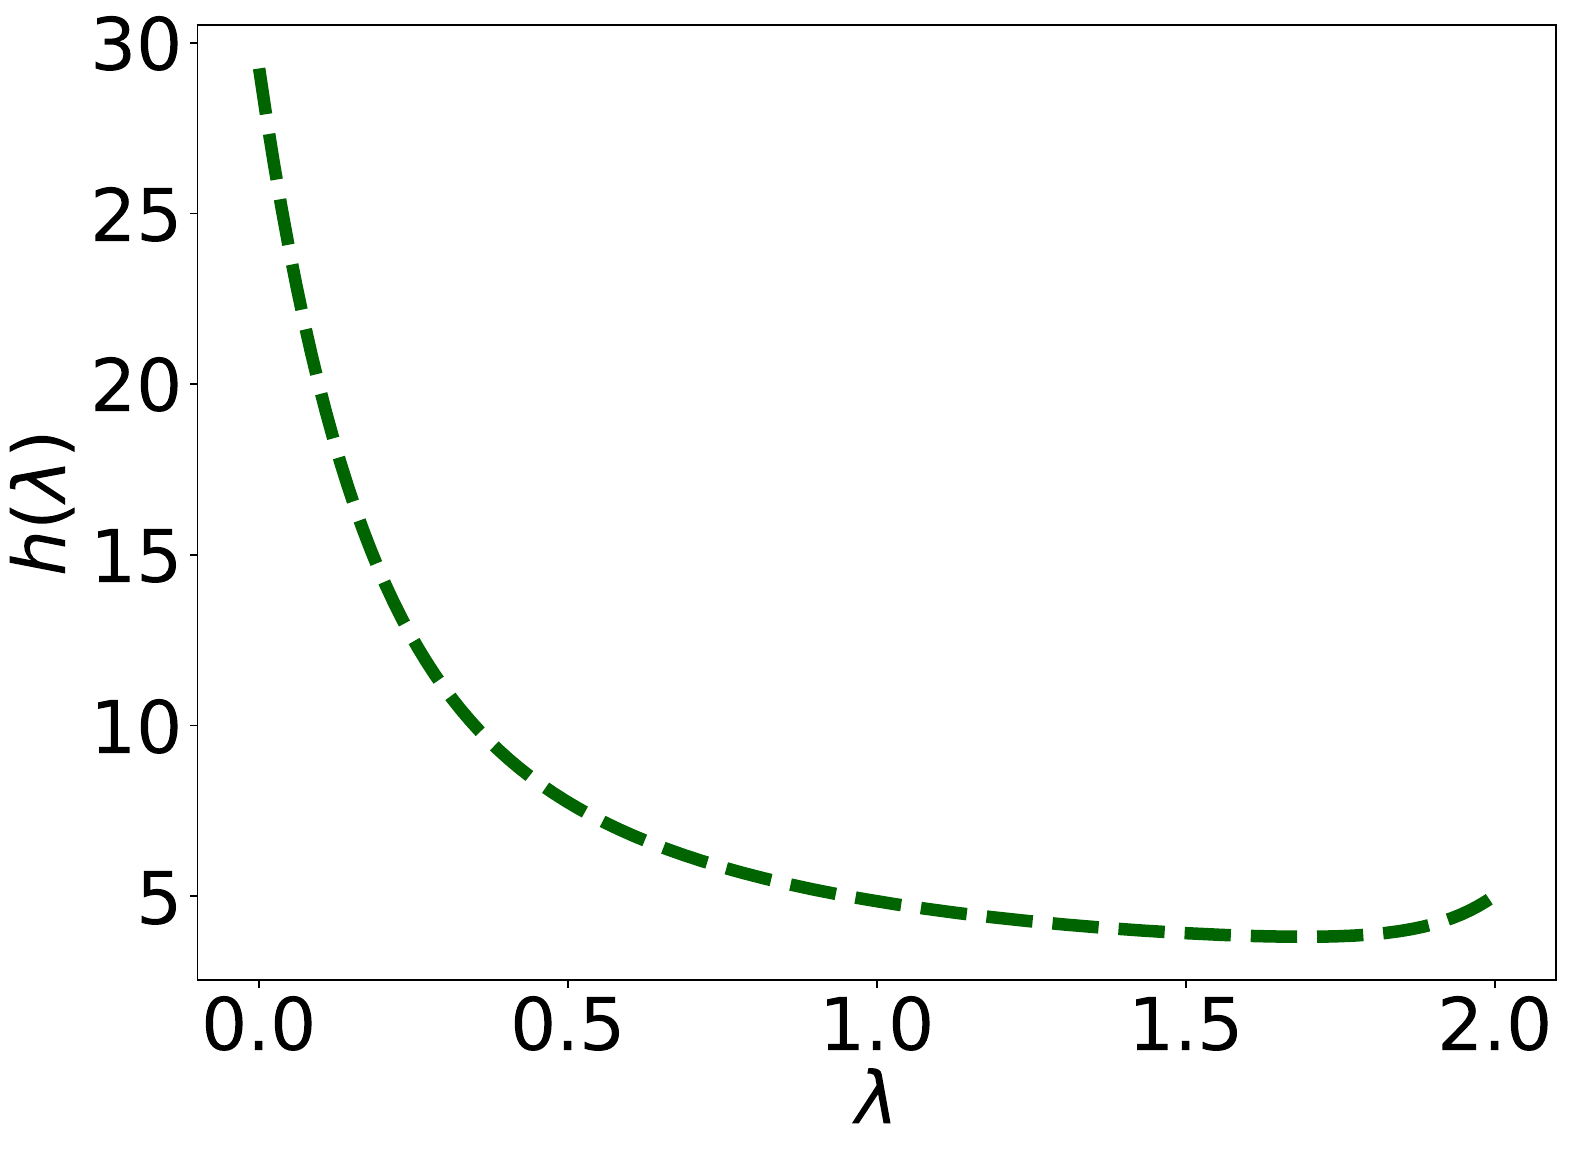}
  % \caption{Filter of UniFilter}
  \caption{UniFilter on Pubmed}
  \label{fig:image1}
\end{subfigure}%
\begin{subfigure}{0.22\textwidth}
  \centering
  \includegraphics[width=\linewidth]{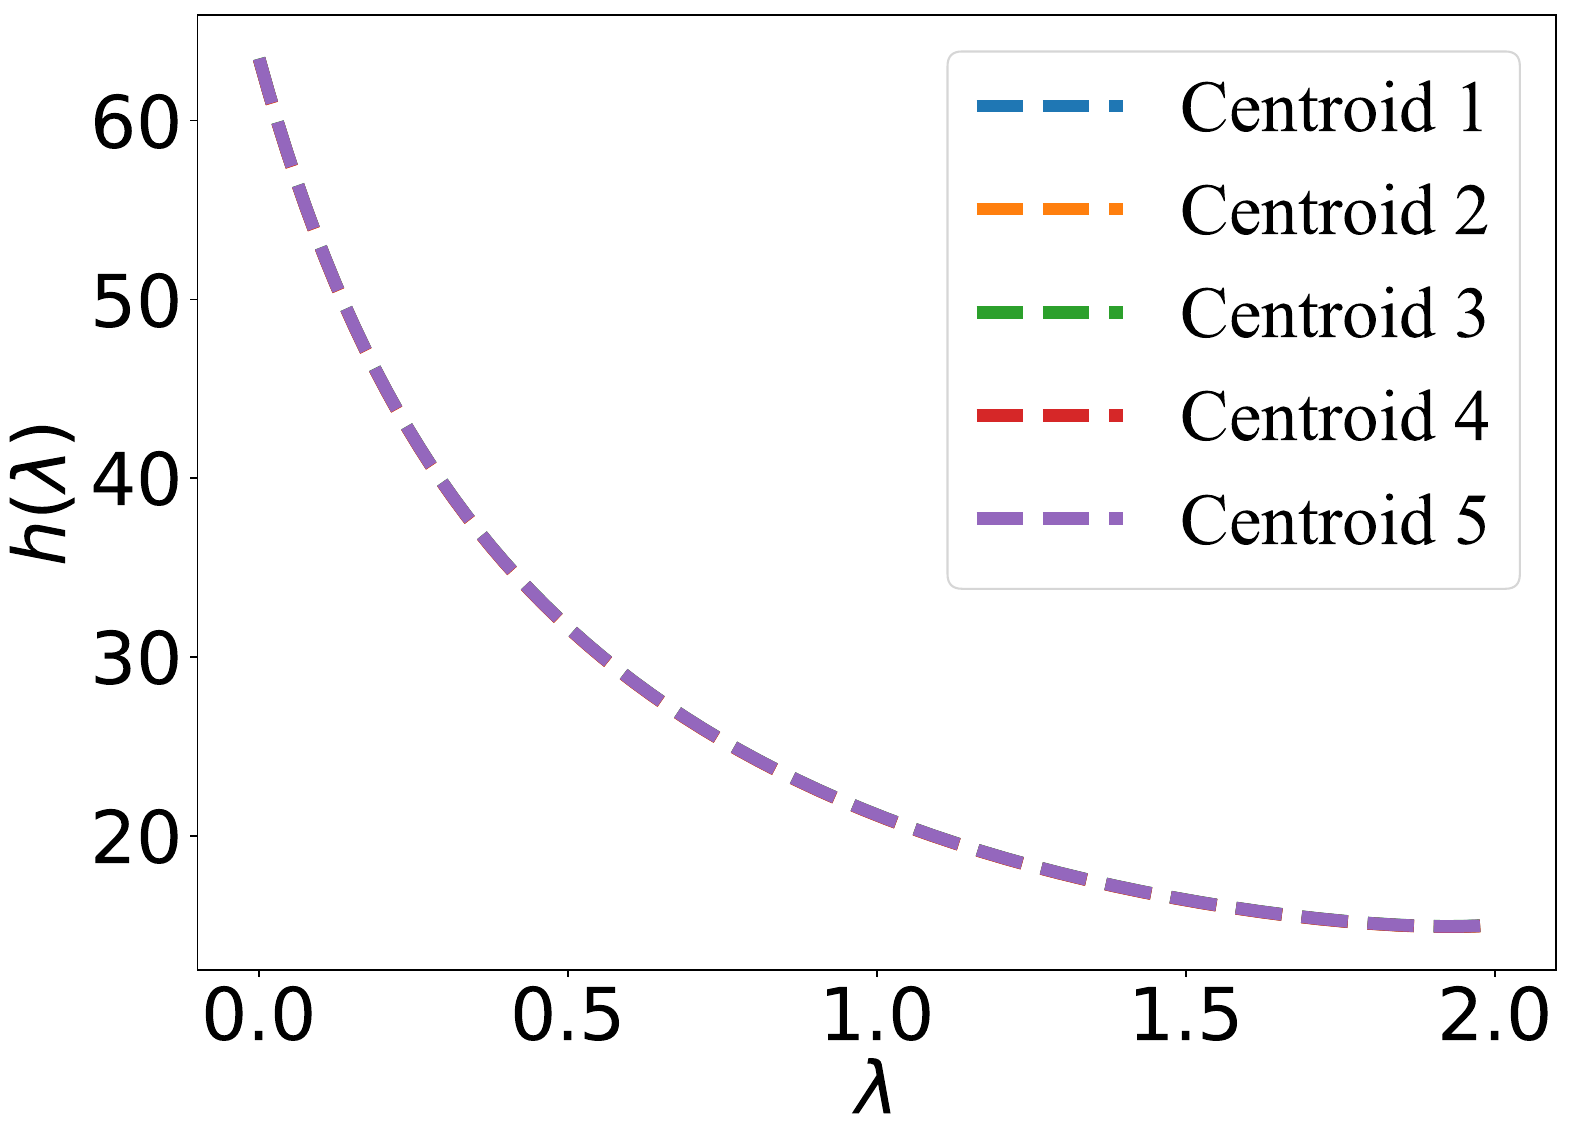}
  % \caption{Filters of PolyAttn}
  \caption{PolyAttn on Pubmed}
  \label{fig:image2}
\end{subfigure}%
\\
\begin{subfigure}{0.22\textwidth}
  \centering
  \includegraphics[width=\linewidth]{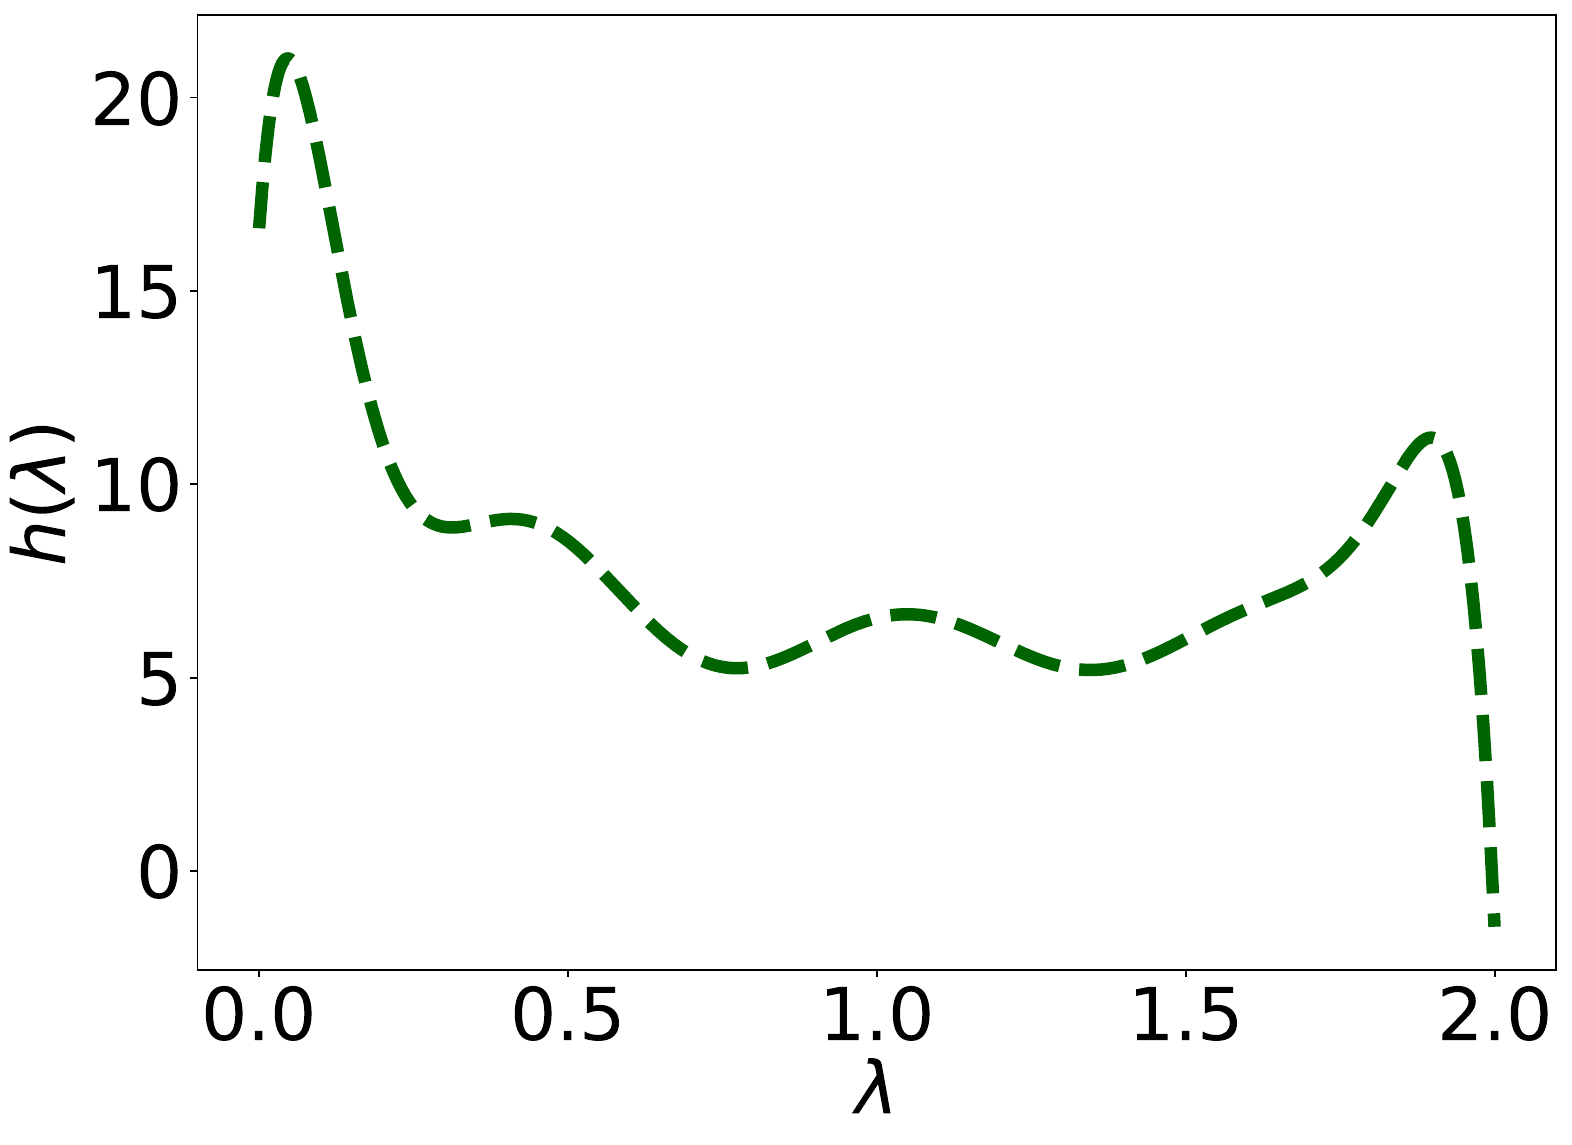}
  % \caption{Filter of UniFilter}
  \caption{UniFilter on Pubmed}
  \label{fig:image3}
\end{subfigure}%
\begin{subfigure}{0.222\textwidth}
  \centering
  \includegraphics[width=\linewidth]{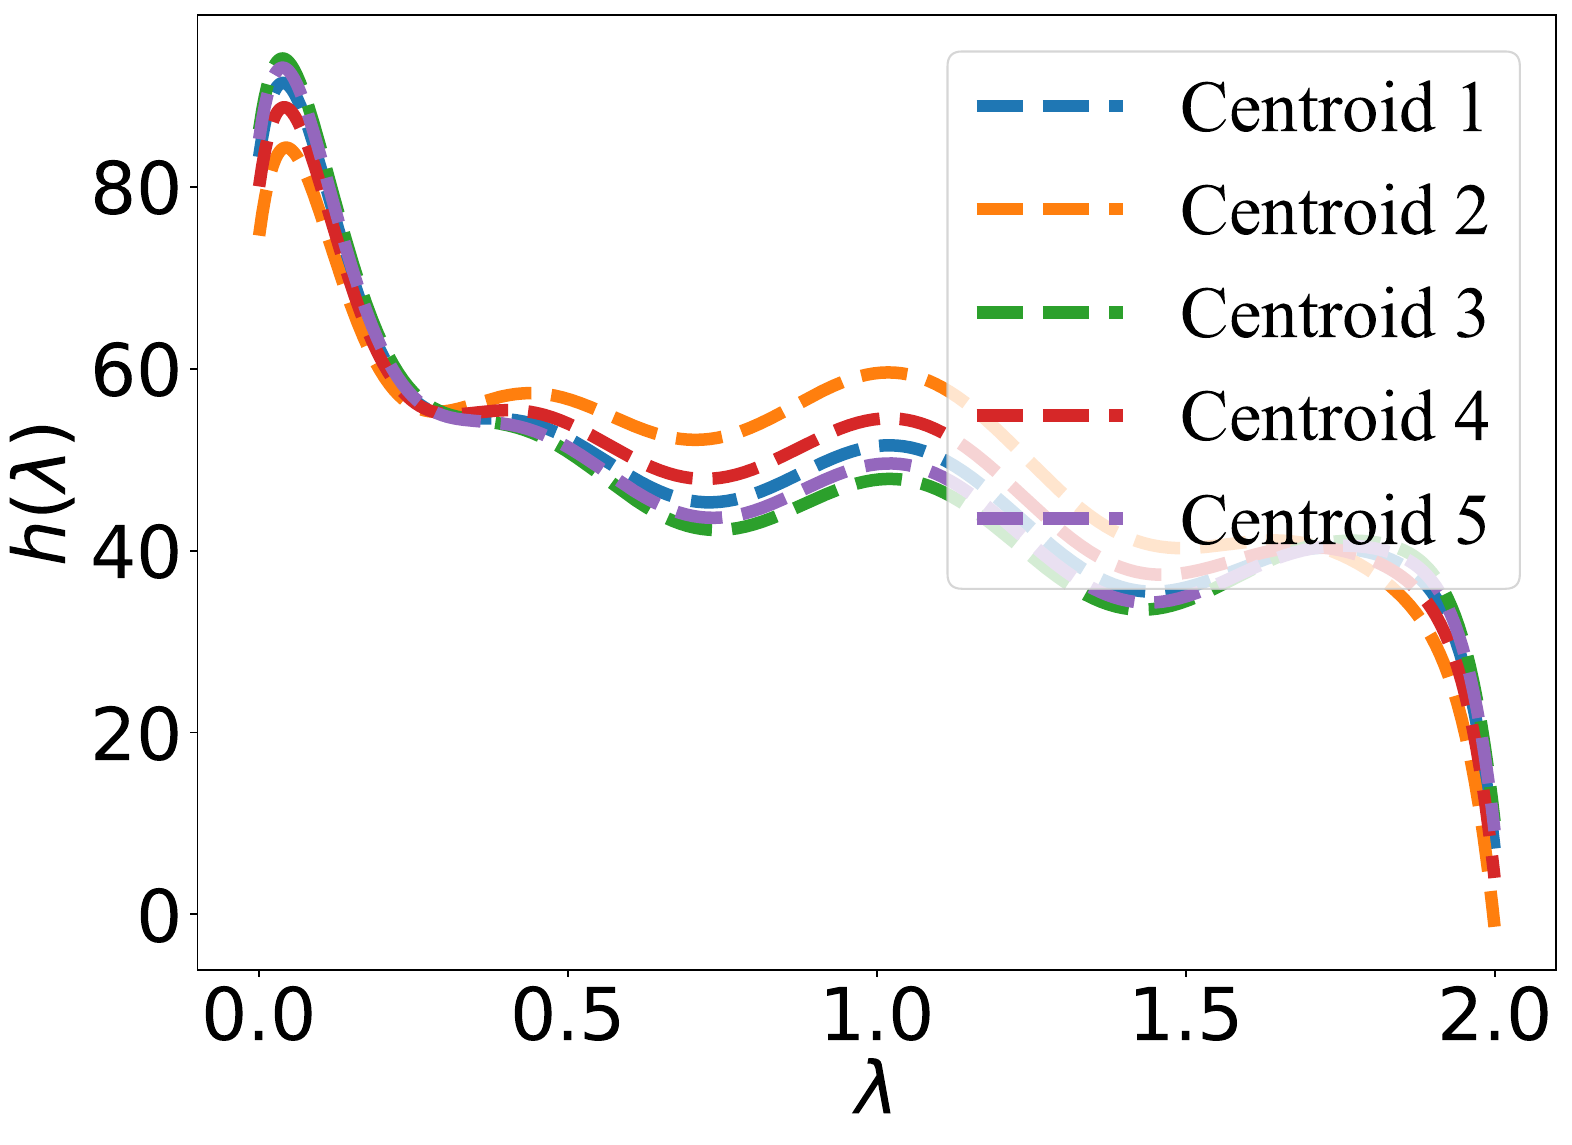}
  % \caption{Filters of PolyAttn}
  \caption{PolyAttn on Pubmed}
  \label{fig:image4}
\end{subfigure}%
\vspace{-3mm}
\caption{Filters Learned on \textbf{Pubmed} (\textit{Monomial basis} at the top and \textit{Chebyshev basis} at the bottom).}
\label{app_fig1}
\end{figure}
% \vspace{-4mm}

\begin{figure}[htbp]
\centering
\begin{subfigure}{0.23\textwidth}
  \centering
  \includegraphics[width=\linewidth]{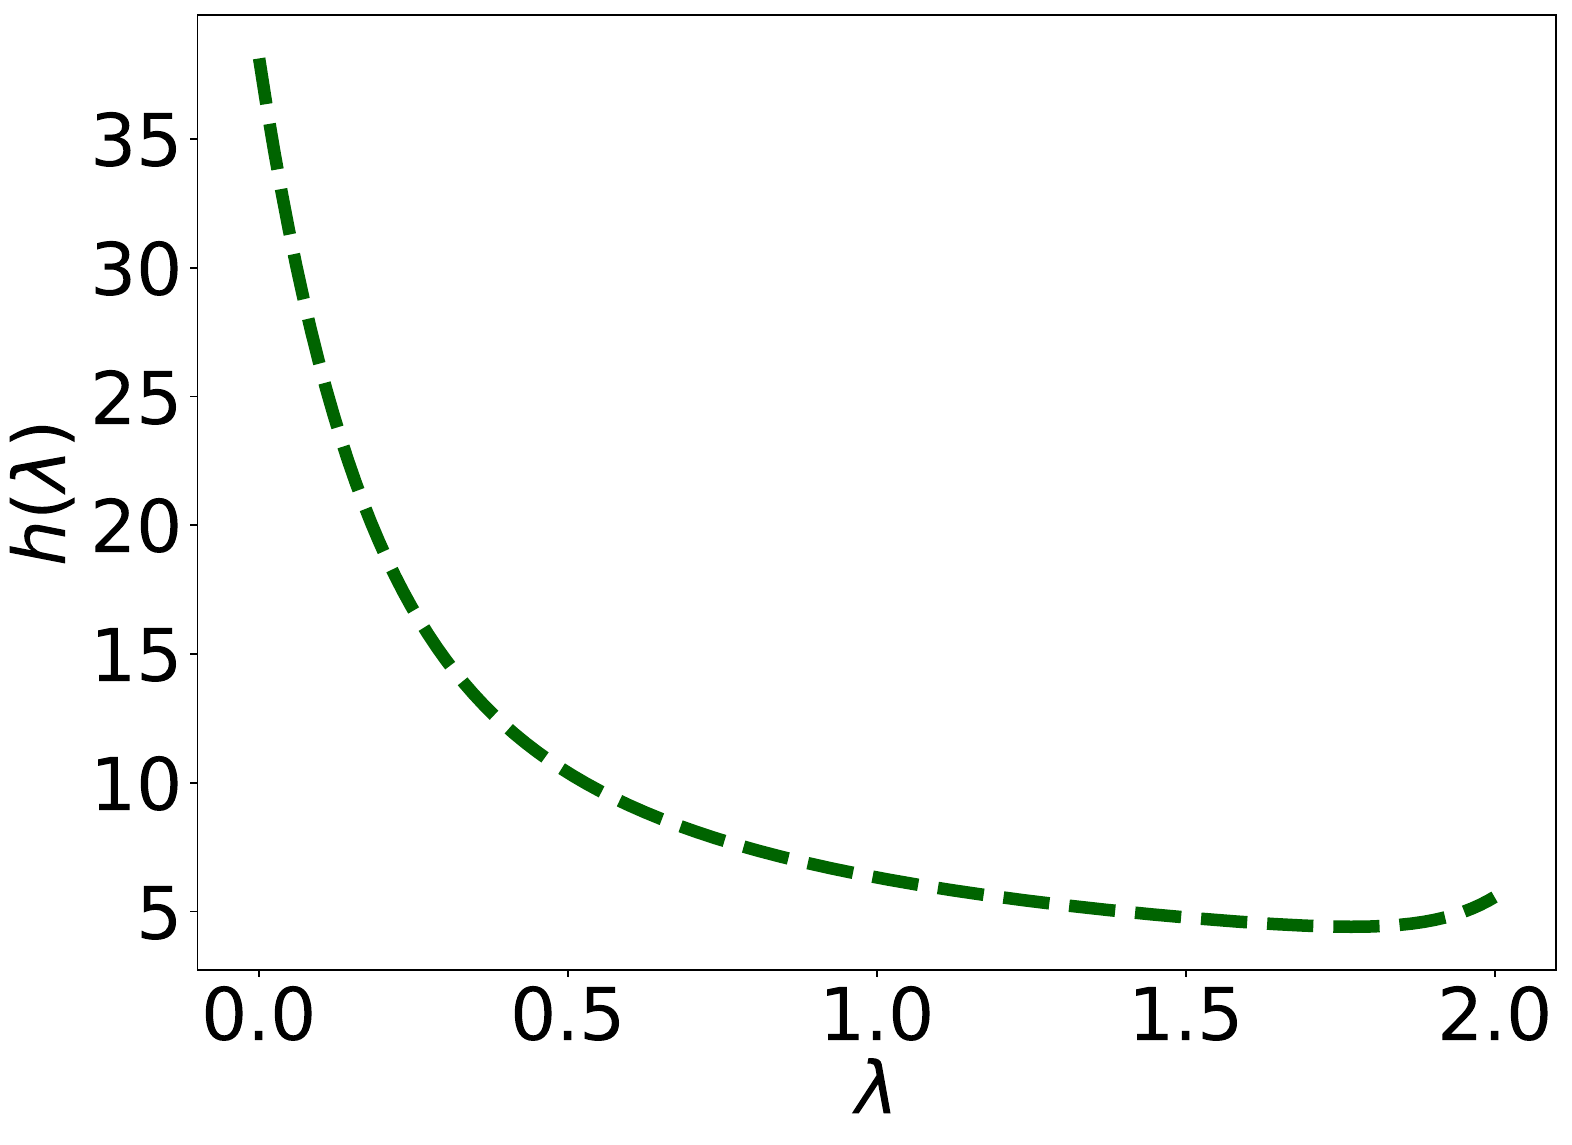}
  % \caption{Filter of UniFilter}
  \caption{UniFilter on CS}
  \label{fig:image1}
\end{subfigure}%
\begin{subfigure}{0.23\textwidth}
  \centering
  \includegraphics[width=\linewidth]{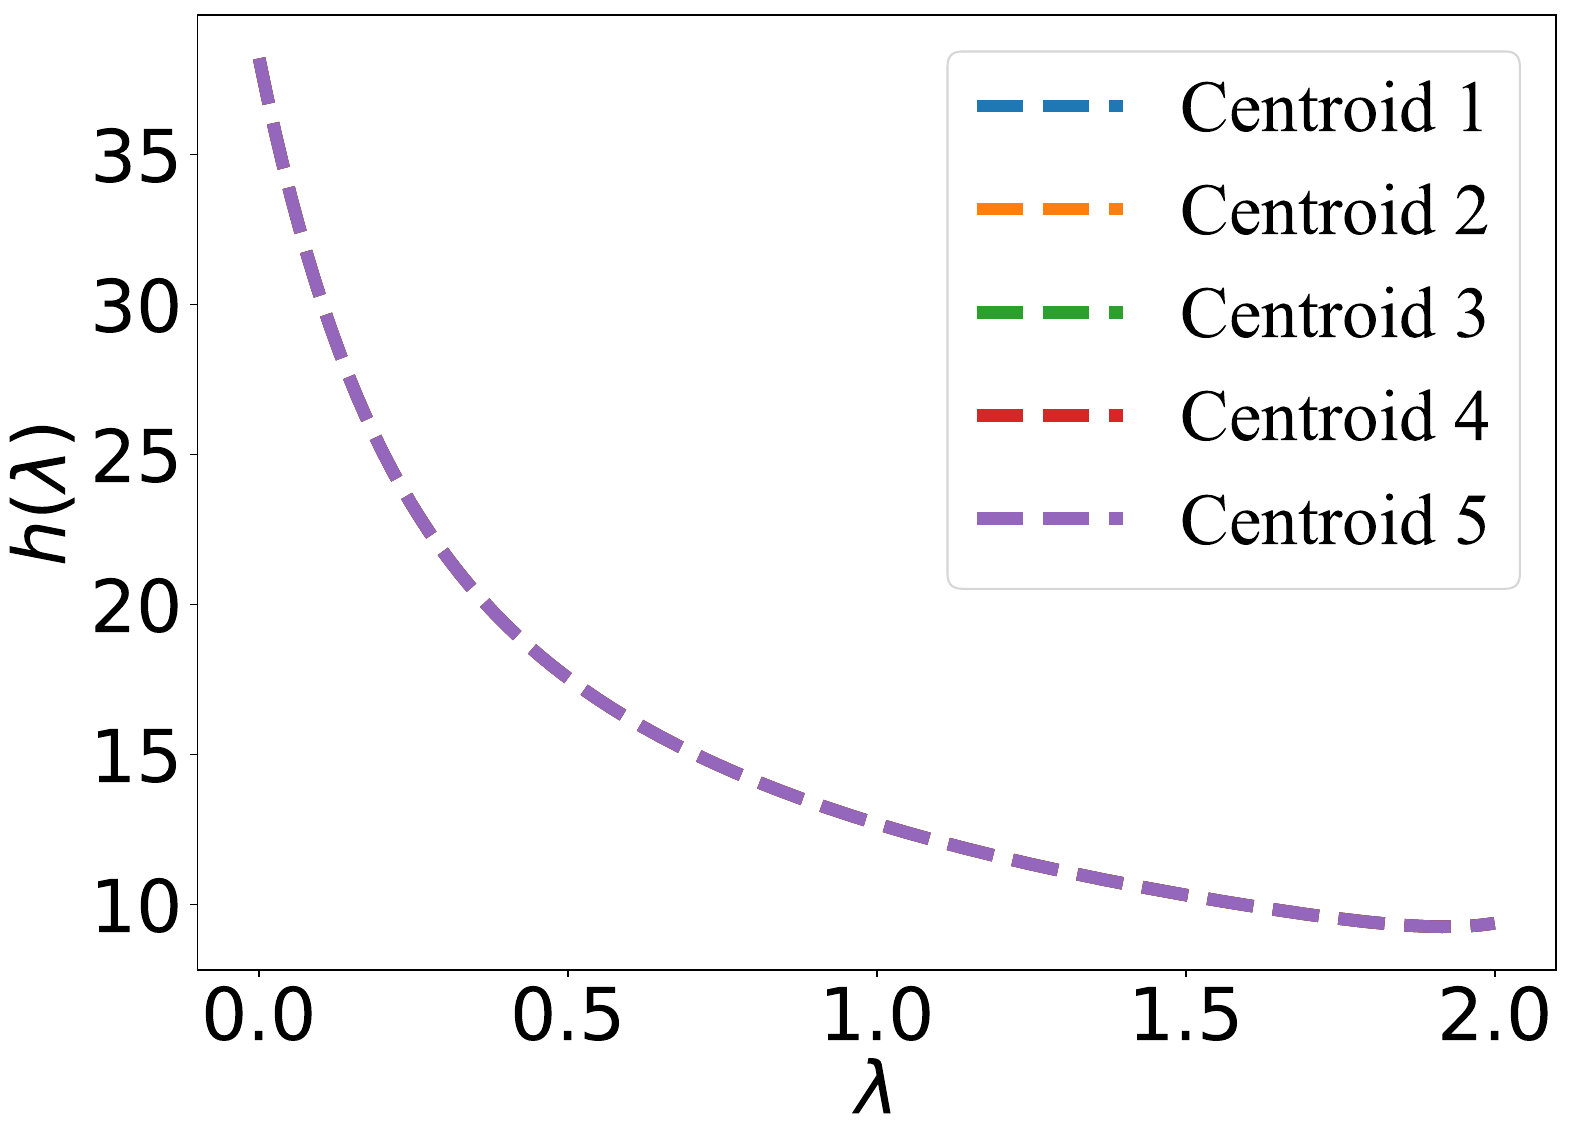}
  % \caption{Filters of PolyAttn}
  \caption{PolyAttn on CS}
  \label{fig:image2}
\end{subfigure}%
\\
\begin{subfigure}{0.22\textwidth}
  \centering
  \includegraphics[width=\linewidth]{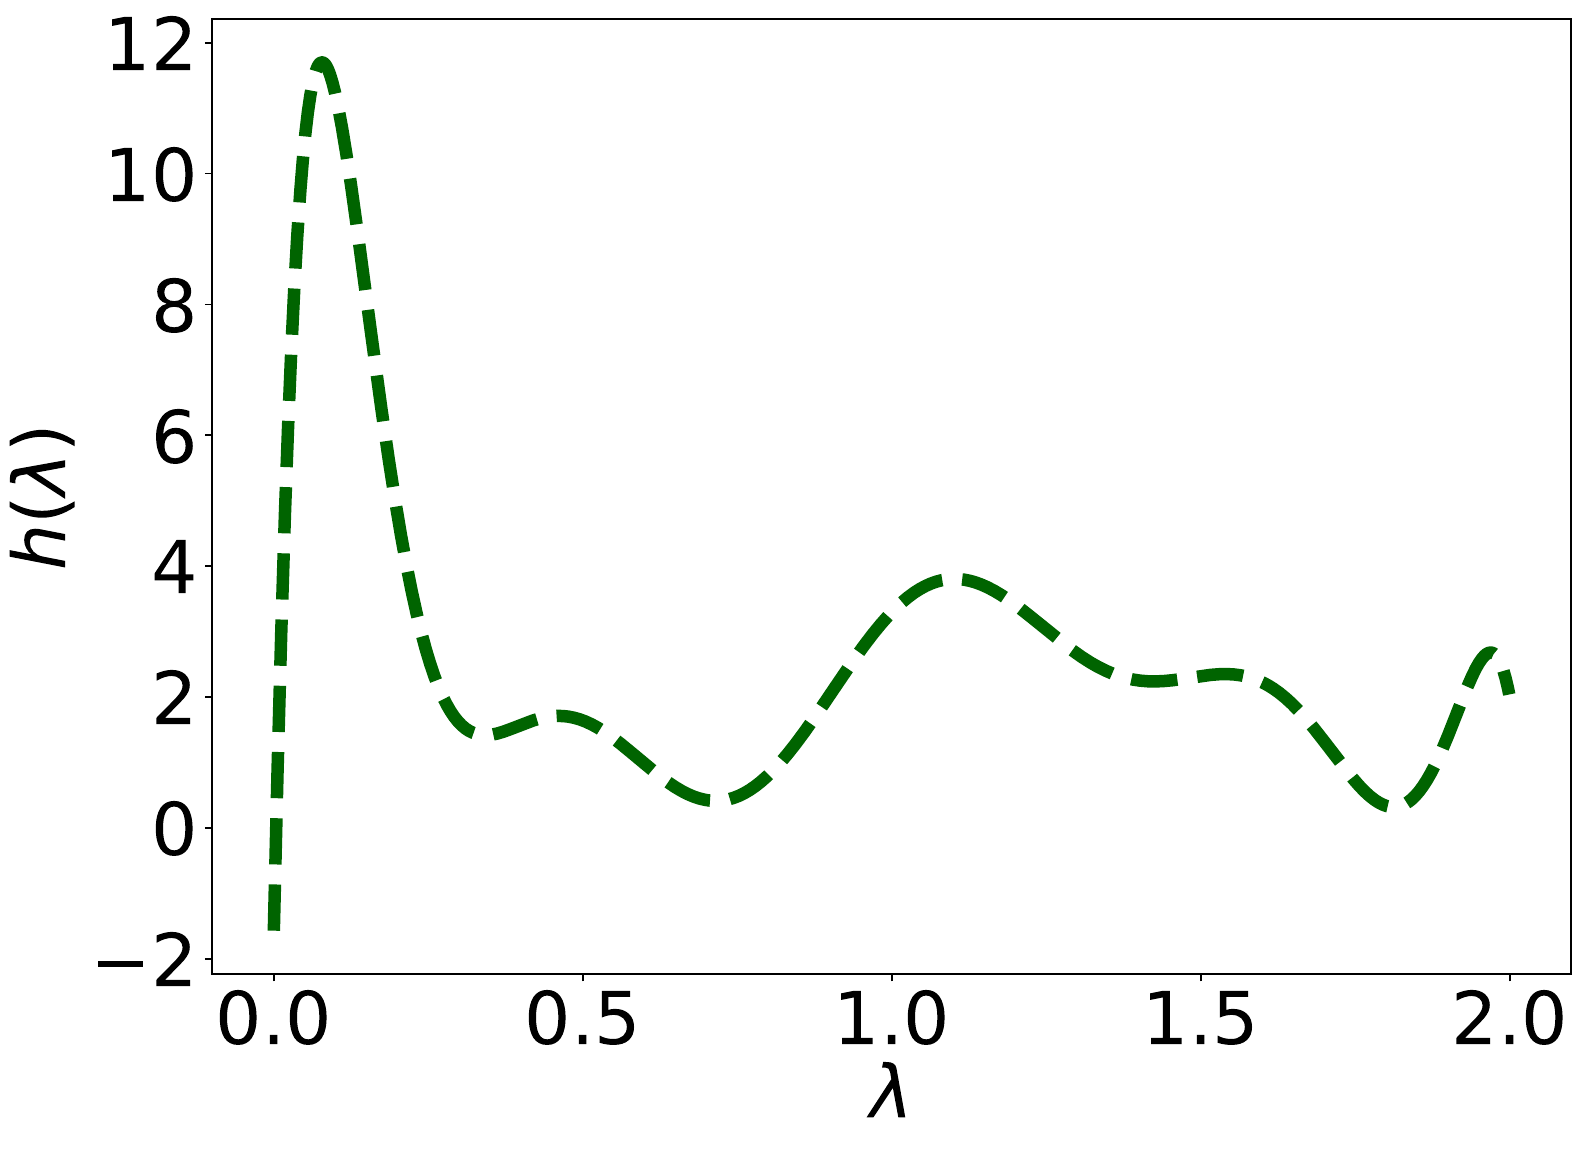}
  % \caption{Filter of UniFilter}
  \caption{UniFilter on CS}
  \label{fig:image3}
\end{subfigure}%
\begin{subfigure}{0.22\textwidth}
  \centering
  \includegraphics[width=\linewidth]{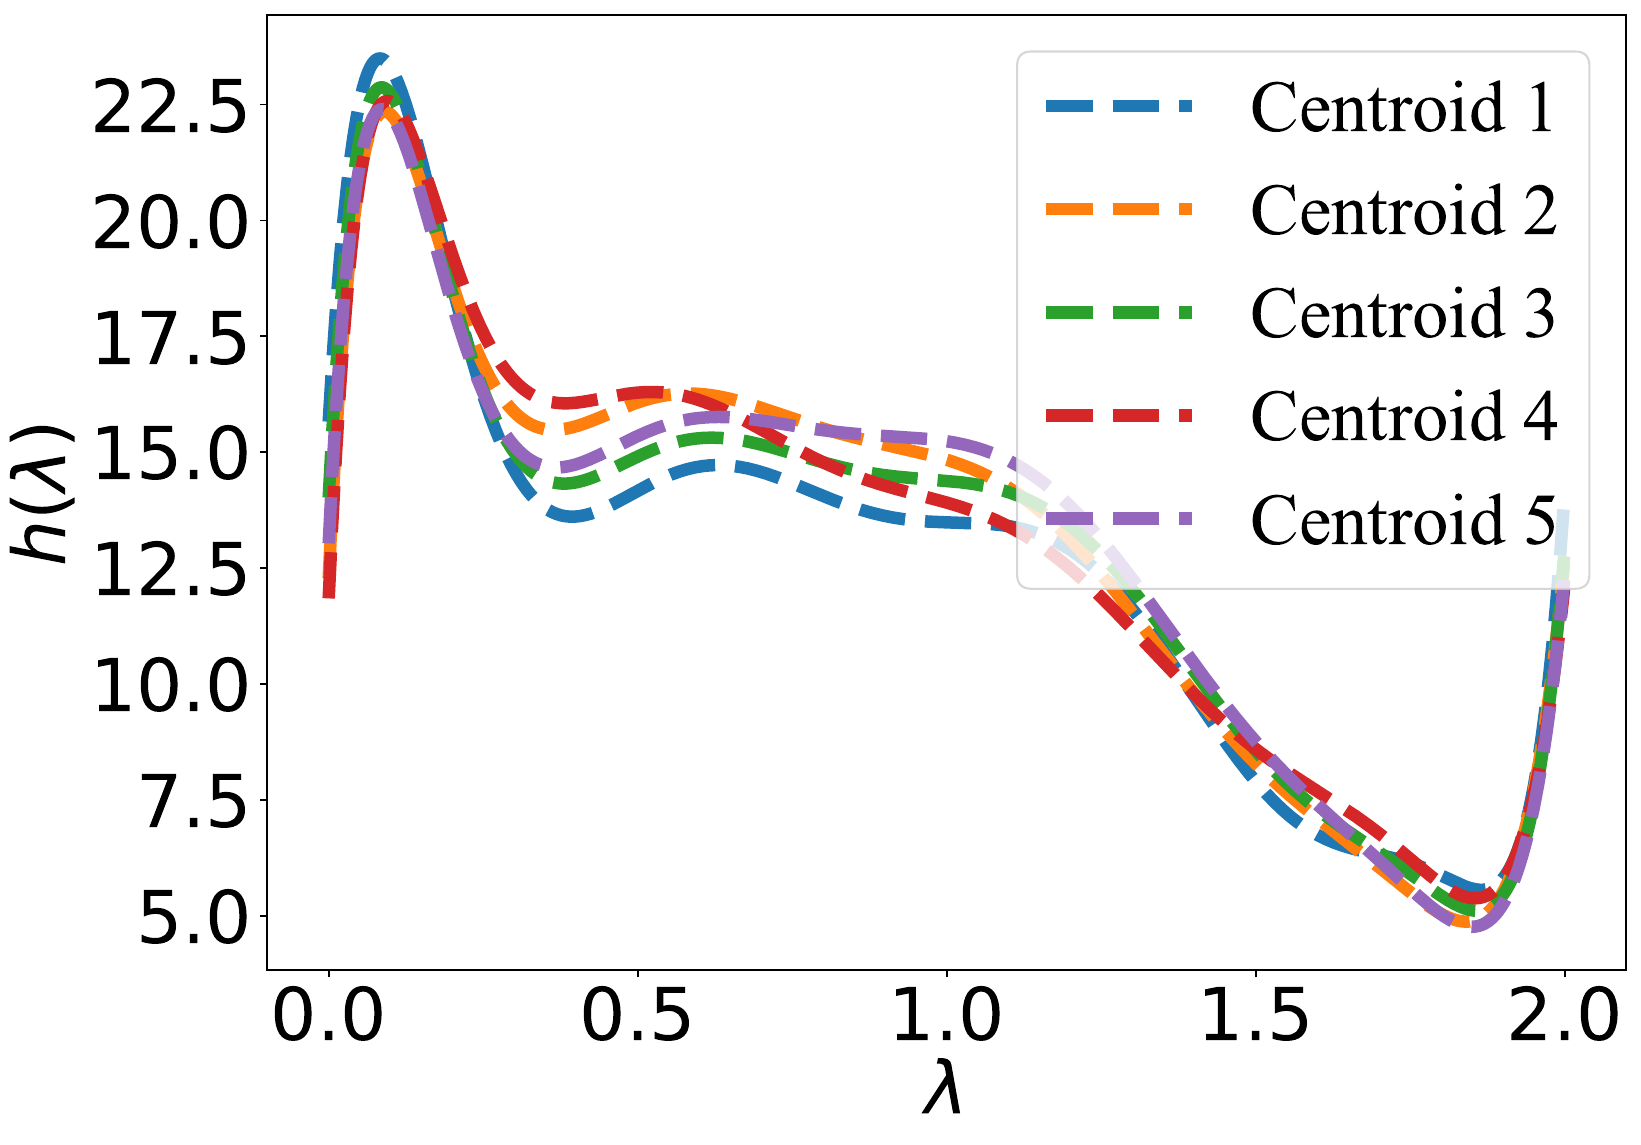}
  % \caption{Filters of PolyAttn}
  \caption{PolyAttn on CS}
  \label{fig:image4}
\end{subfigure}%
\vspace{-3mm}
\caption{Filters Learned on \textbf{CS} (\textit{Monomial basis} at the top and \textit{Chebyshev basis} at the bottom).}
\label{app_fig2}
\end{figure}
% \vspace{-4mm}

\begin{figure}[htbp]
\centering
\begin{subfigure}{0.23\textwidth}
  \centering
  \includegraphics[width=\linewidth]{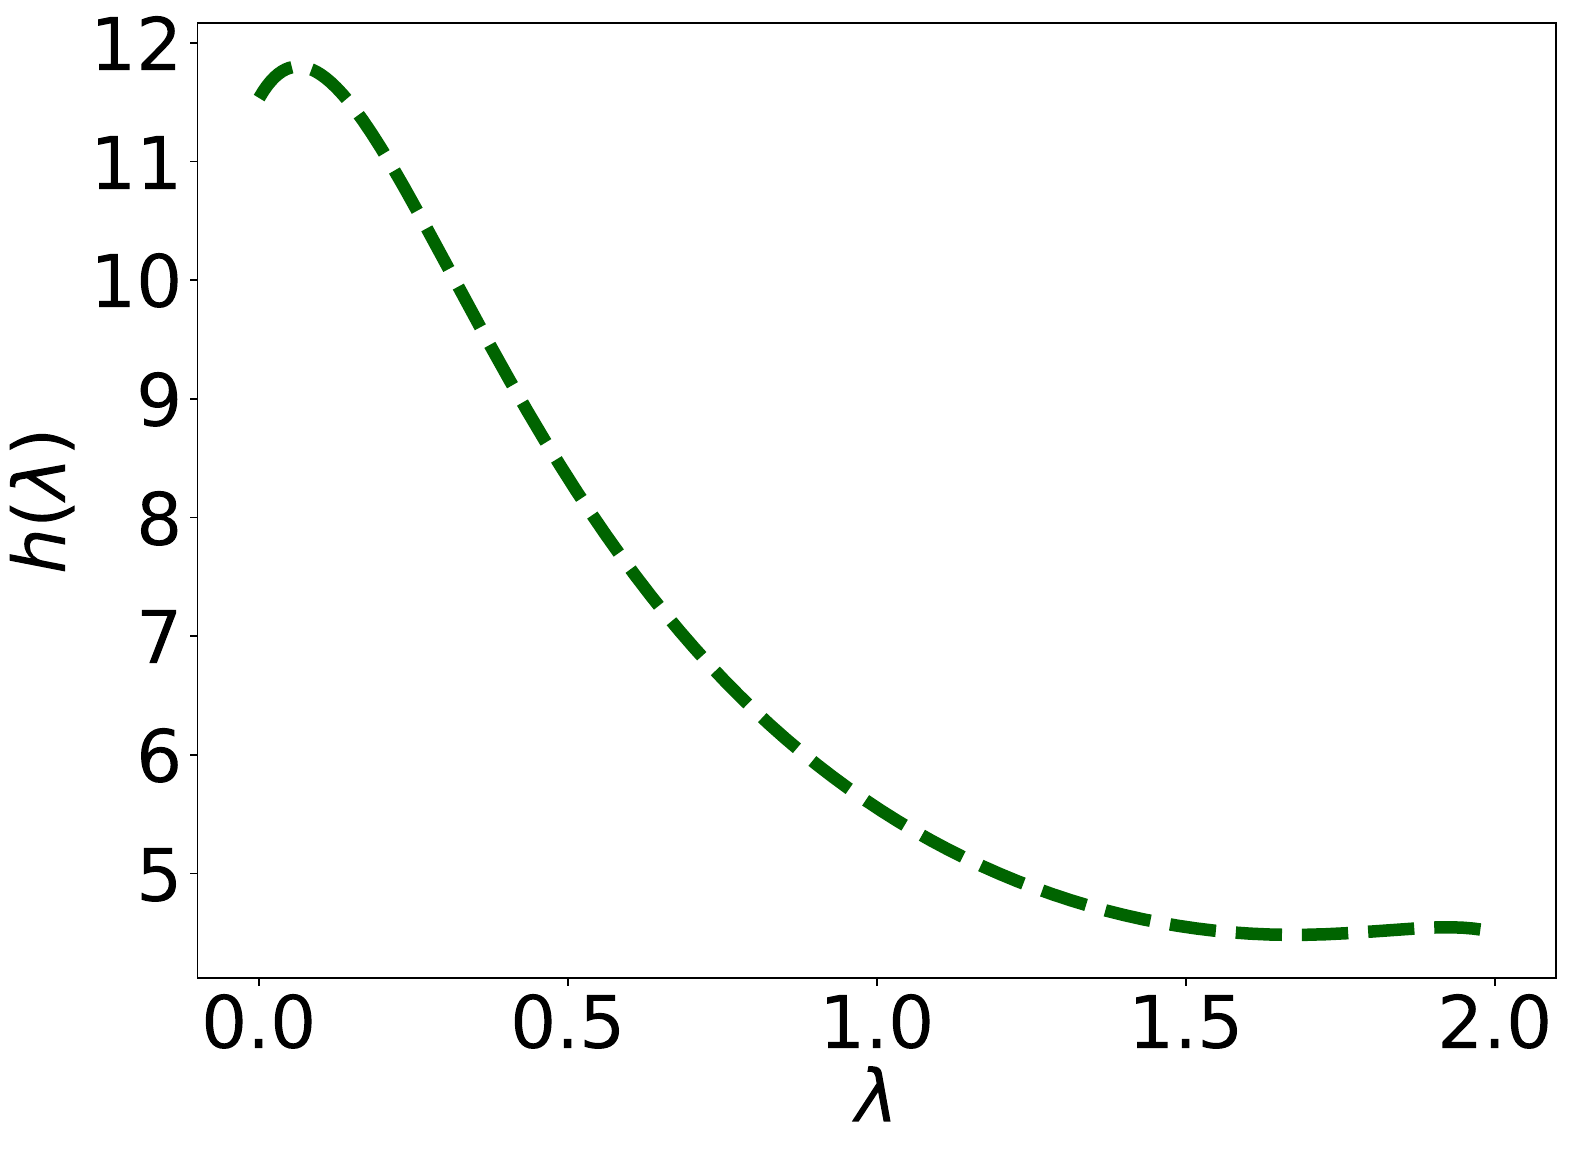}
  % \caption{Filter of UniFilter}
  \caption{UniFilter on Roman-empire}
  \label{fig:image1}
\end{subfigure}%
\begin{subfigure}{0.23\textwidth}
  \centering
  \includegraphics[width=\linewidth]{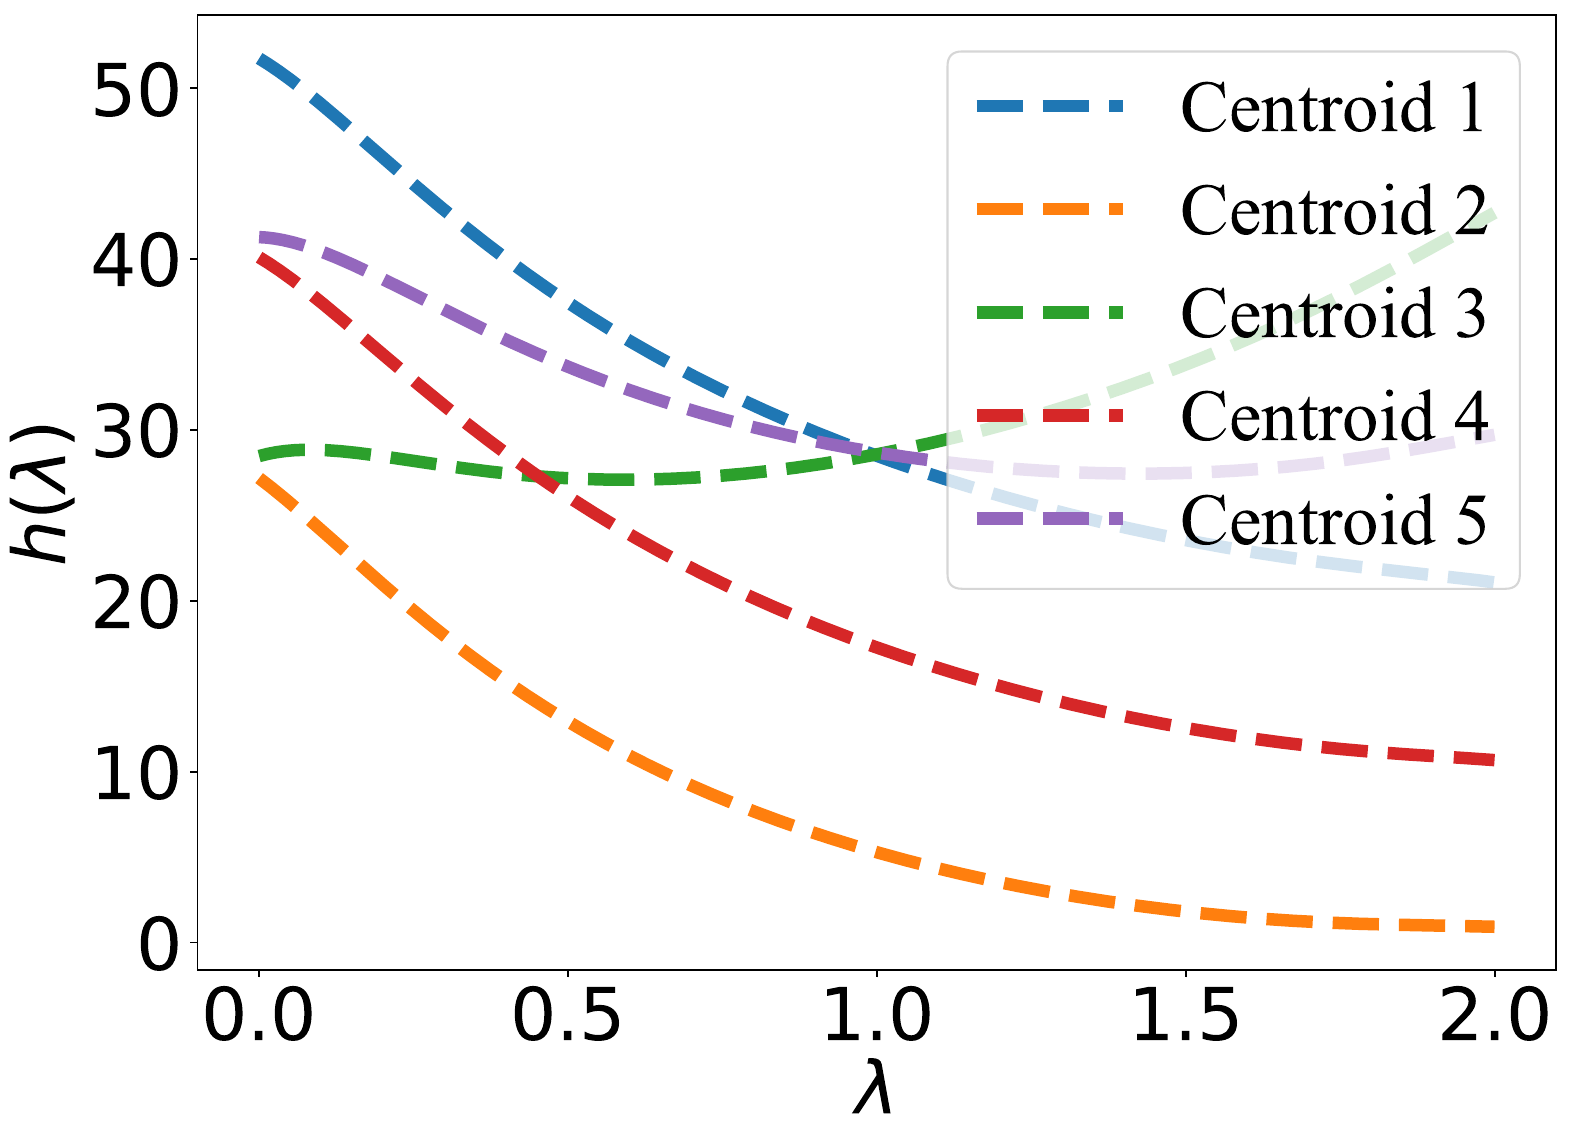}
  % \caption{Filters of PolyAttn}
  \caption{PolyAttn on Roman-empire}
  \label{fig:image2}
\end{subfigure}%
\\
\begin{subfigure}{0.22\textwidth}
  \centering
  \includegraphics[width=\linewidth]{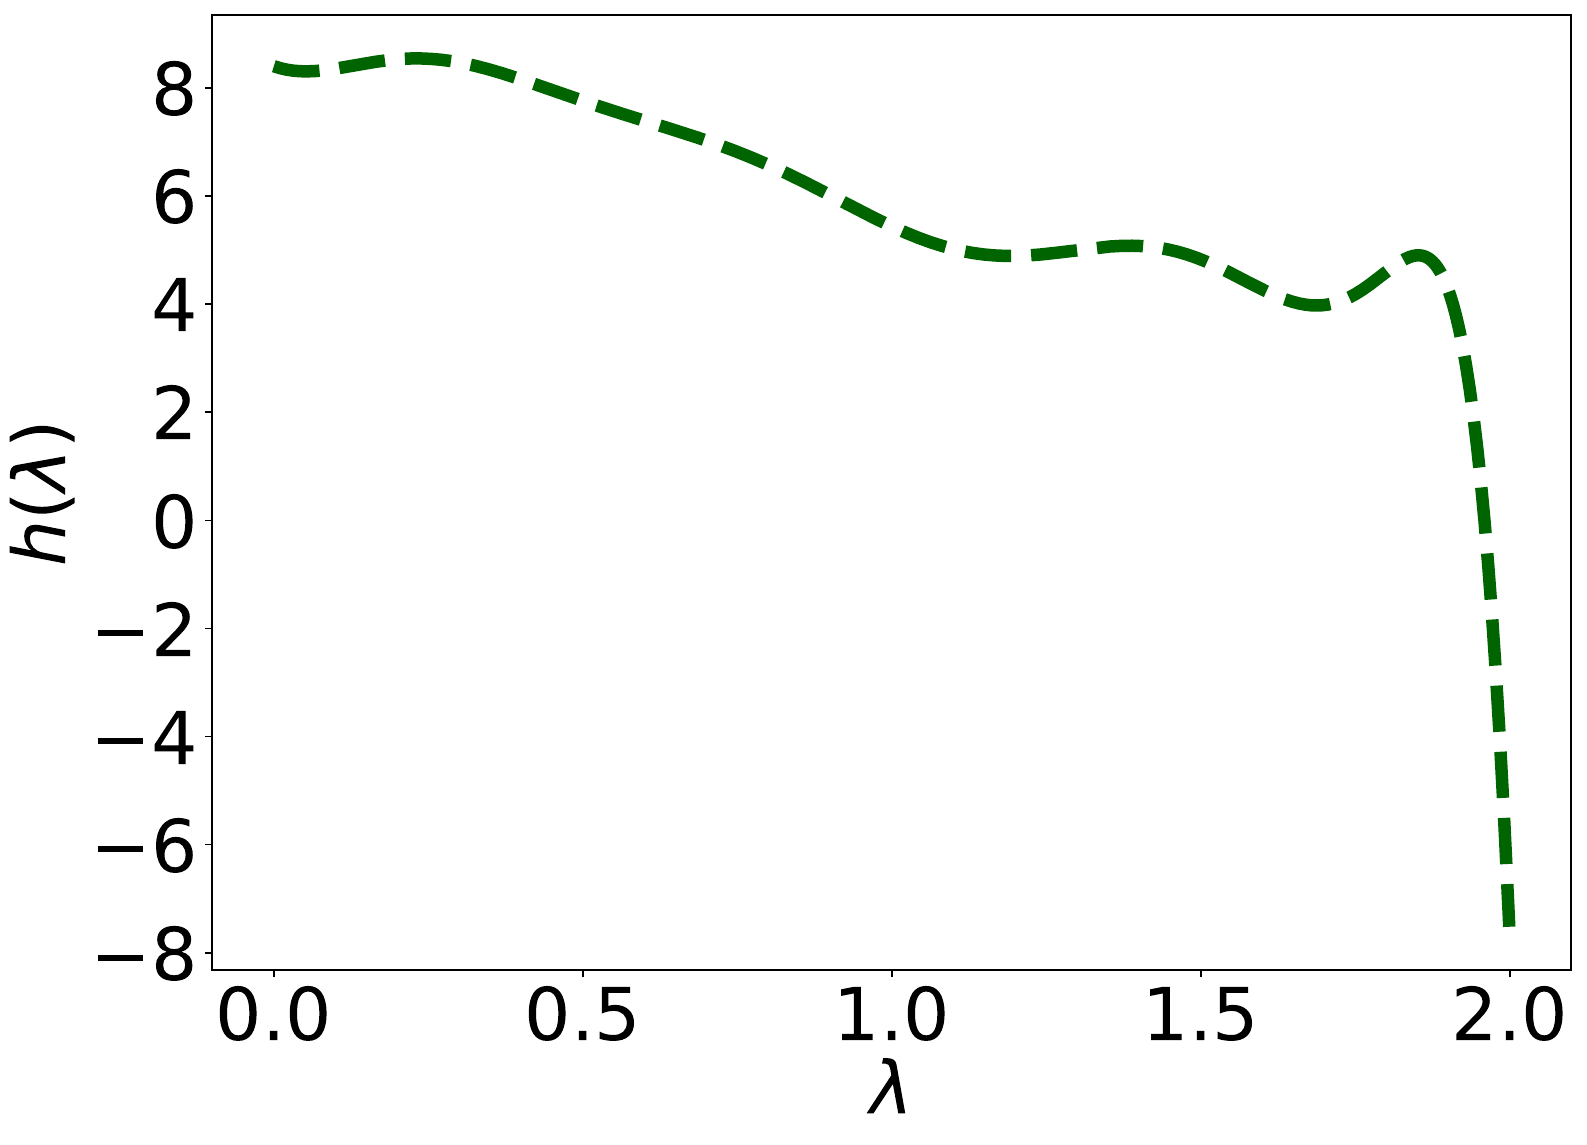}
  % \caption{Filter of UniFilter}
  \caption{UniFilter on Roman-empire}
  \label{fig:image3}
\end{subfigure}%
\begin{subfigure}{0.22\textwidth}
  \centering
  \includegraphics[width=\linewidth]{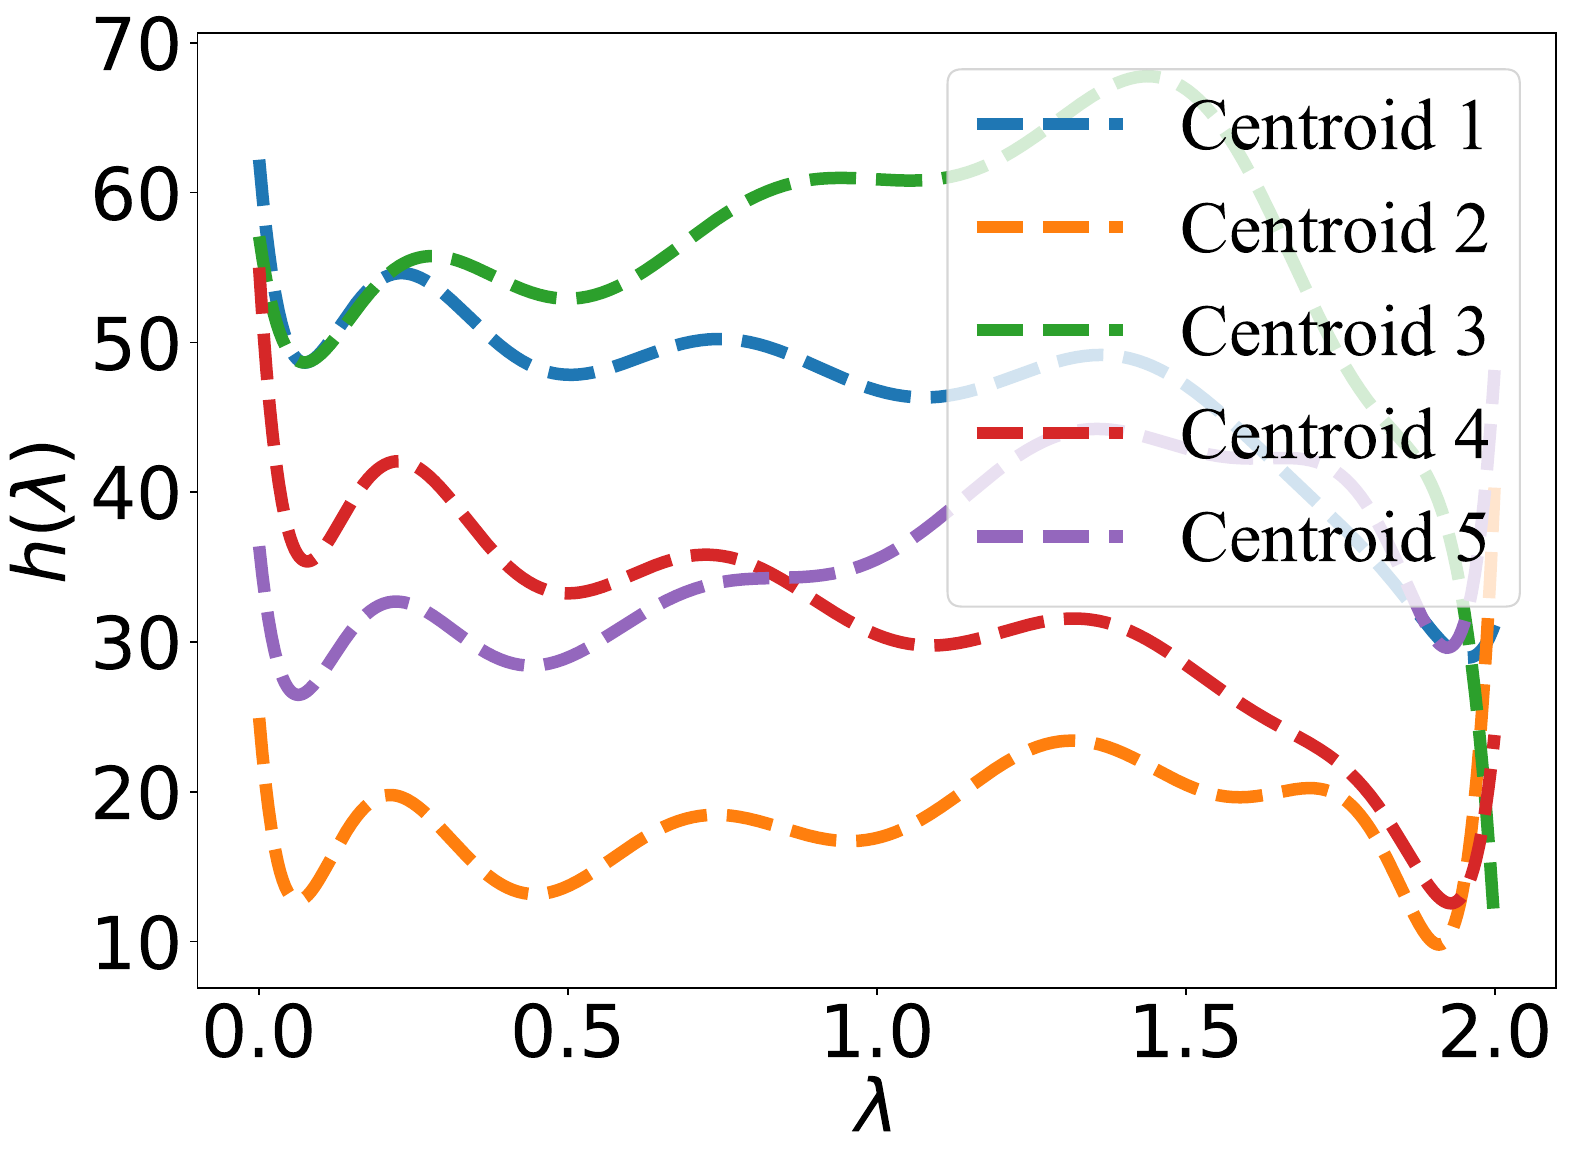}
  % \caption{Filters of PolyAttn}
  \caption{PolyAttn on Roman-empire}
  \label{fig:image4}
\end{subfigure}%
\vspace{-3mm}
\caption{Filters Learned on \textbf{Roman-empire} (\textit{Monomial basis} at the top and \textit{Chebyshev basis} at the bottom).}
\label{app_fig3}
\end{figure}
% \vspace{-4mm}

\begin{figure}[htbp]
\centering
\begin{subfigure}{0.23\textwidth}
  \centering
  \includegraphics[width=\linewidth]{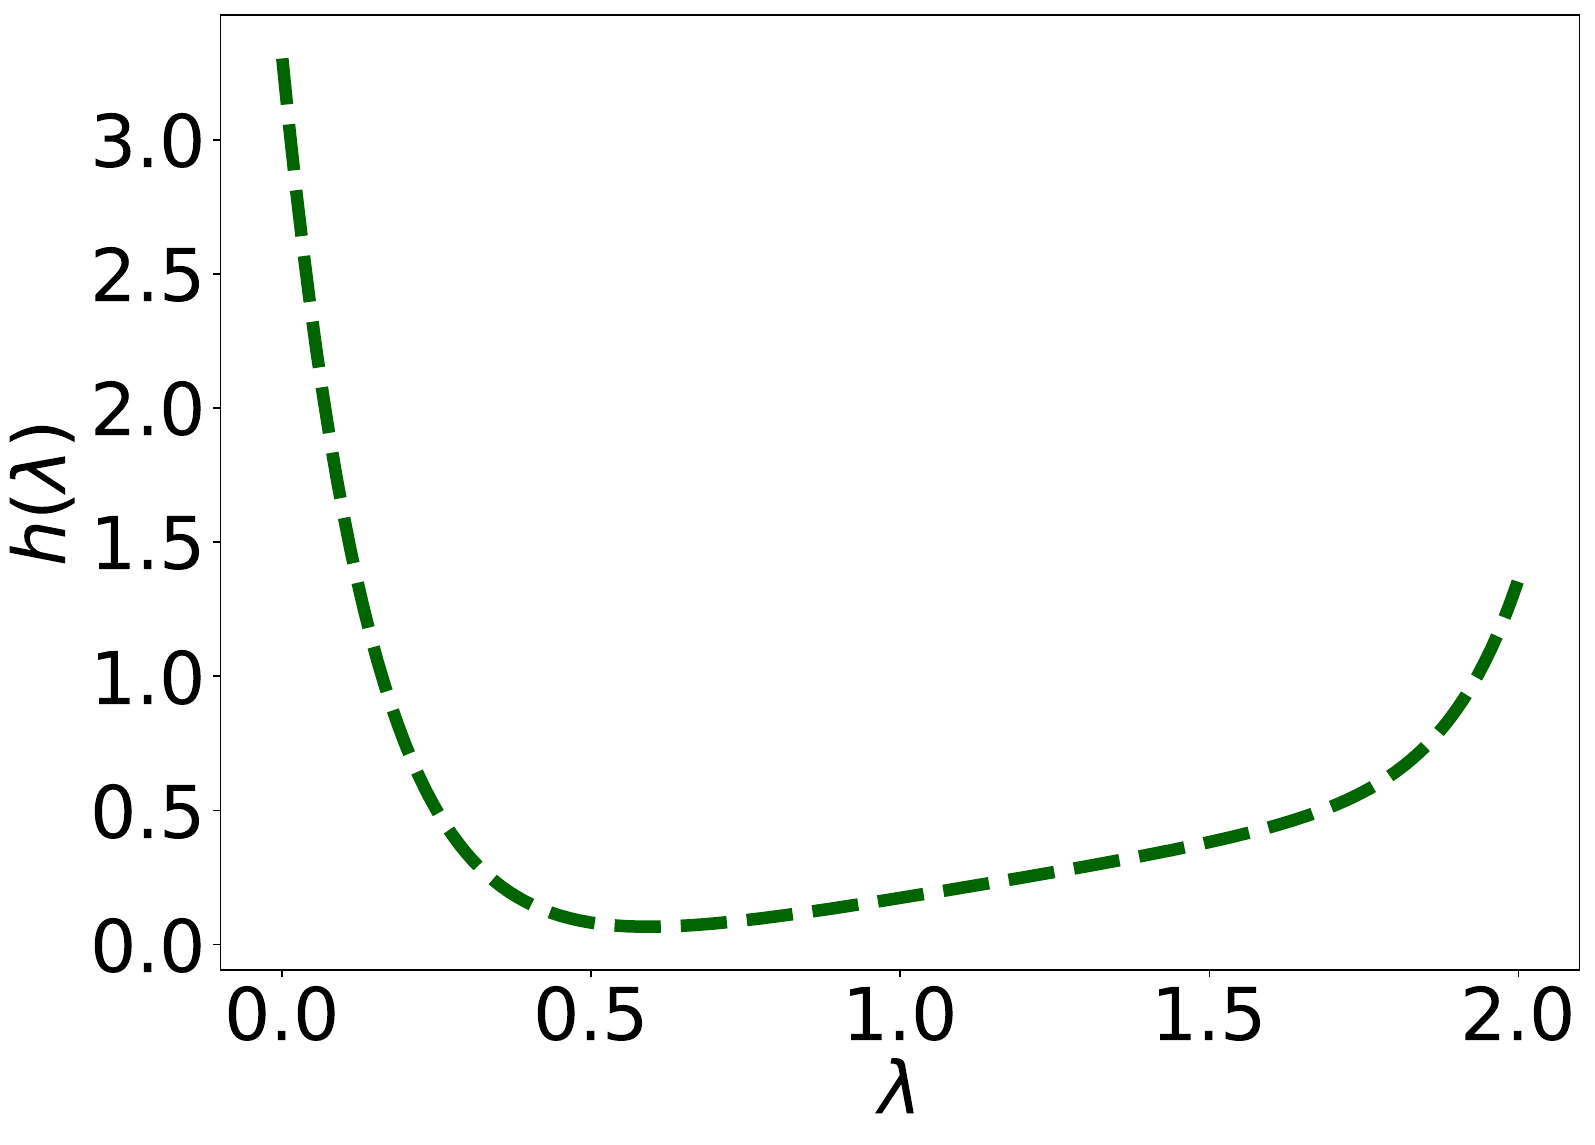}
  % \caption{Filter of UniFilter}
  \caption{UniFilter on Questions}
  \label{fig:image1}
\end{subfigure}%
\begin{subfigure}{0.23\textwidth}
  \centering
  \includegraphics[width=\linewidth]{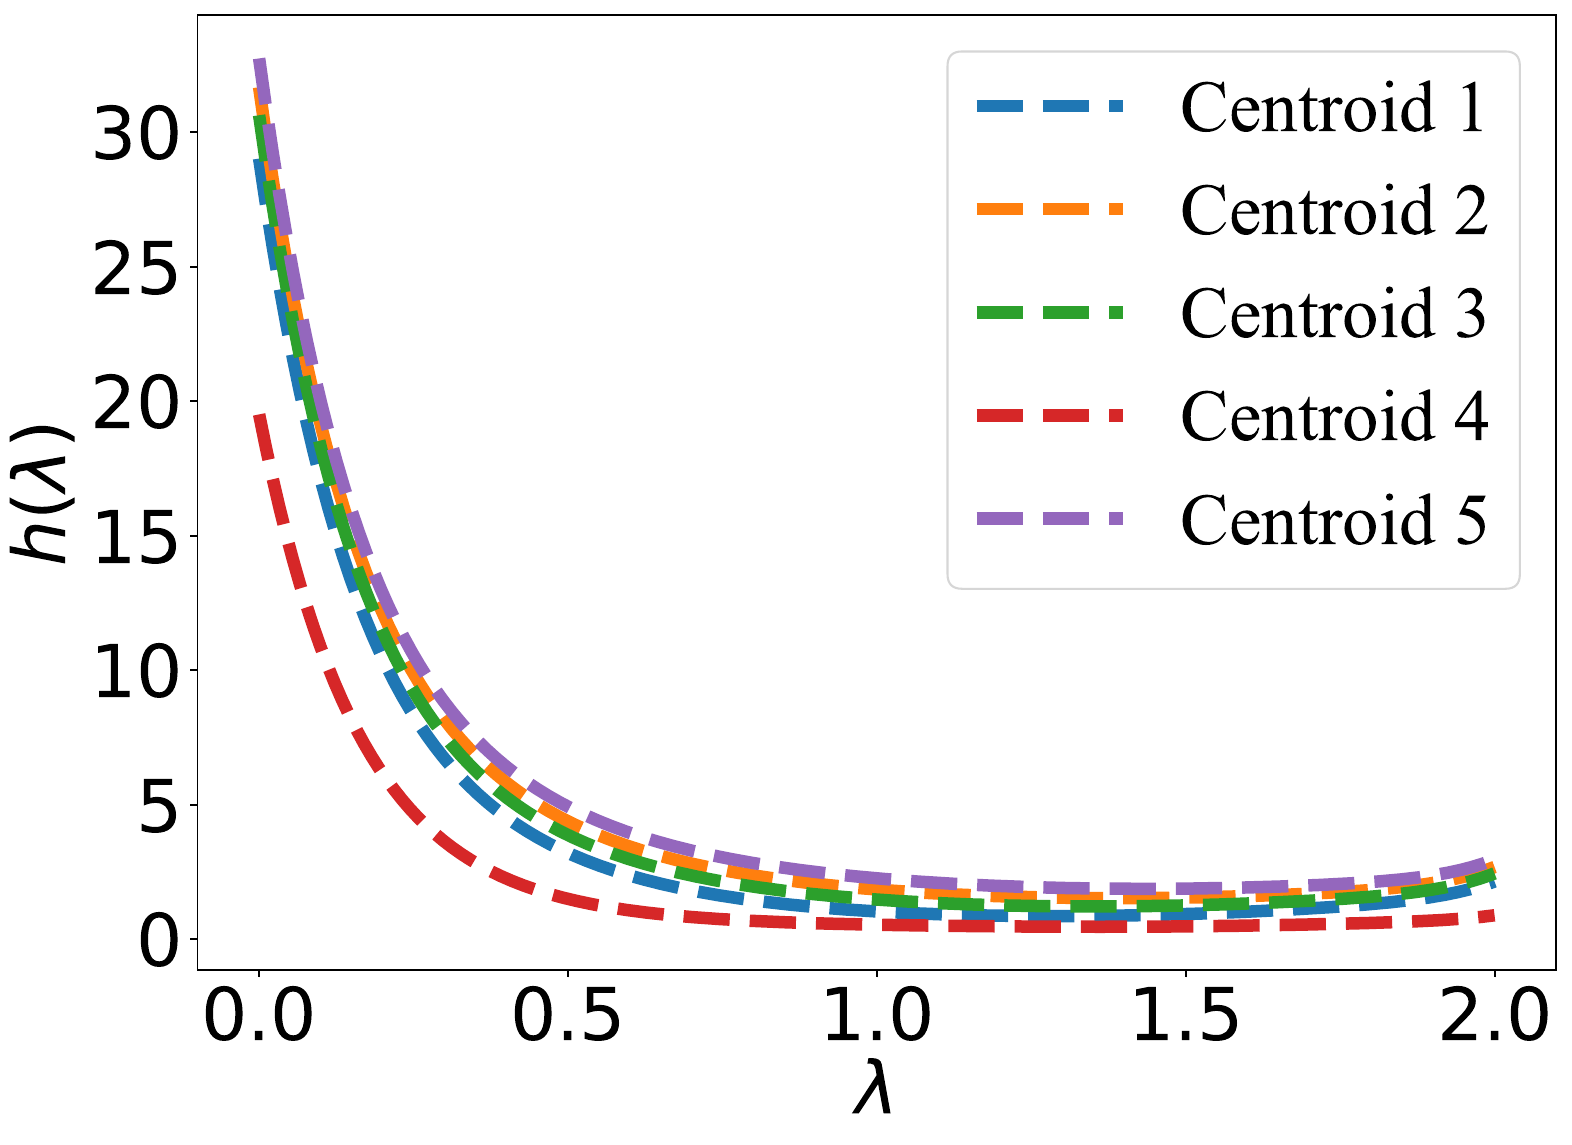}
  % \caption{Filters of PolyAttn}
  \caption{PolyAttn on Questions}
  \label{fig:image2}
\end{subfigure}%
\\
\begin{subfigure}{0.22\textwidth}
  \centering
  \includegraphics[width=\linewidth]{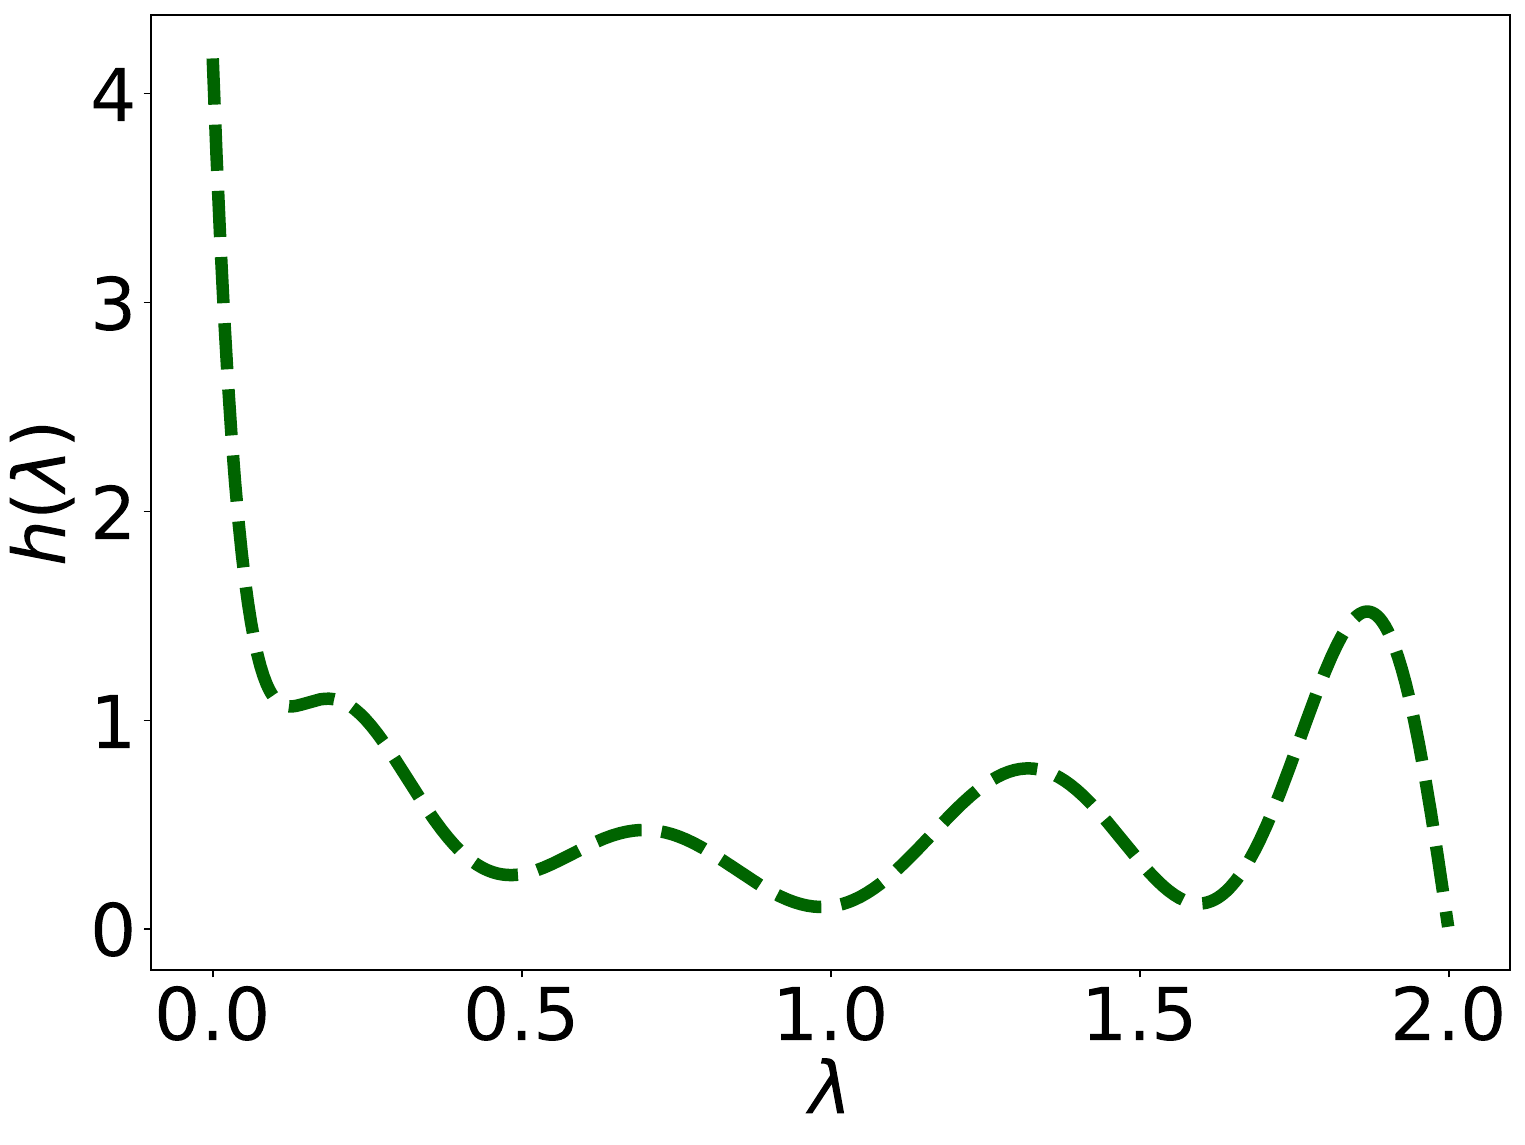}
  % \caption{Filter of UniFilter}
  \caption{UniFilter on Questions}
  \label{fig:image3}
\end{subfigure}%
\begin{subfigure}{0.232\textwidth}
  \centering
  \includegraphics[width=\linewidth]{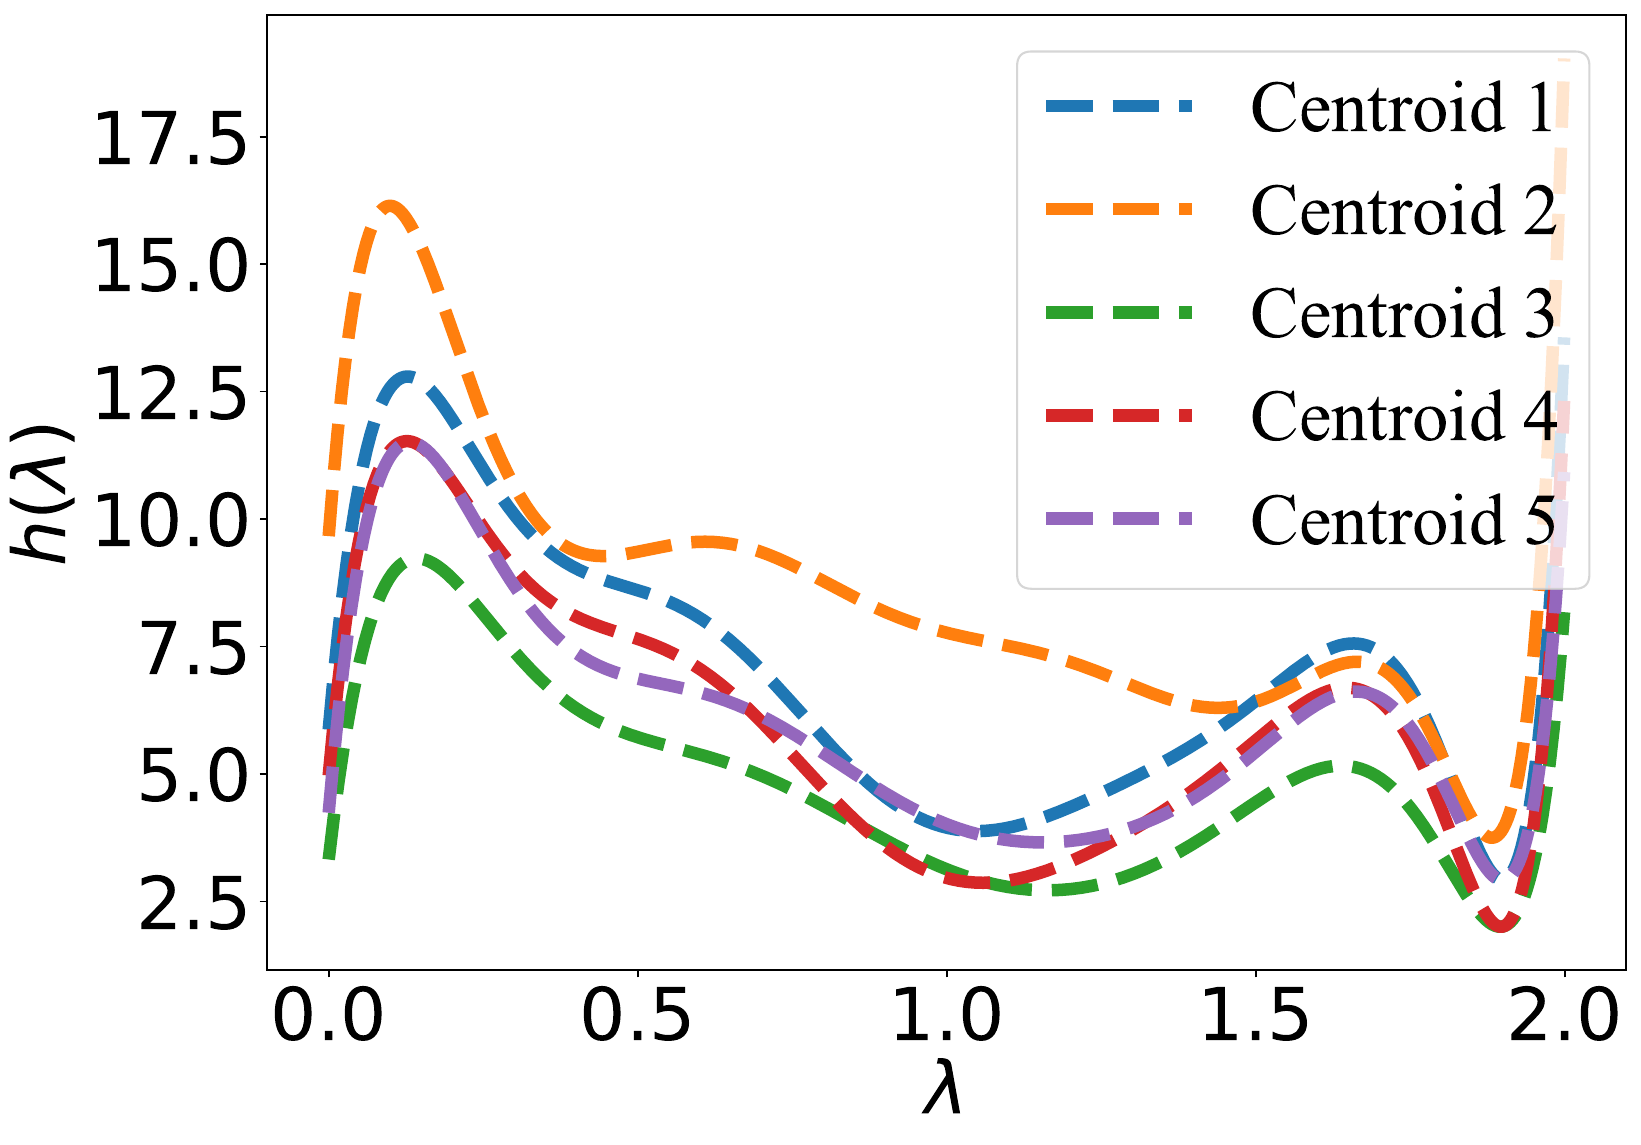}
  % \caption{Filters of PolyAttn}
  \caption{PolyAttn on Questions}
  \label{fig:image4}
\end{subfigure}% 
% \caption{Filters Learned on \textbf{Questions} (\textit{Monomial basis}, top and \textit{Chebyshev basis}, bottom).}
\vspace{-3mm}
\caption{Filters Learned on \textbf{Questions} (\textit{Monomial basis} at the top and \textit{Chebyshev basis} at the bottom).}
\label{app_fig4}
\end{figure}

As depicted in Figures \ref{app_fig1}, \ref{app_fig2}, \ref{app_fig3} and \ref{app_fig4}, PolyAttn learns node-specific filters, enhancing its expressive capacity over node-unified filters. Particularly in heterophilic datasets, PolyAttn exhibits a discernible diversity in learned filters. Conversely, in homophilic graphs, PolyAttn tends to derive uniform or nearly identical filters across nodes. These findings imply that PolyAttn can dynamically adapt its filters to the unique attributes of each graph.
